# Supplementary material for: A continuous integration and web framework in support of the ATLAS Publication Process
Source: arXiv:2005.06989 source file (2021-01-28)
Supplement: Supplementary file 1 [file Appendix_fencegitlab.tex]

%------------------------------------------------------------------------------
\section{FENCE and \gitlab integration classes}%
\label{app:fence:gitlab}
%------------------------------------------------------------------------------

%------------------------------------------------------------------------------
\subsection{Methods}
\label{app:fence:gitlab:methods}

\begin{lstlisting}
public function get($endPoint, $data = null)
{
    $this->init($endPoint, $data);
    return $this->exec();
}

public function post($endPoint, $data = null)
{
    return $this->execMethod('POST', $endPoint, $data);
}

private function delete($endPoint, $data = null)
{
    return $this->execMethod('DELETE', $endPoint, $data);
}

private function put($endPoint, $data = null)
{
    return $this->execMethod('PUT', $endPoint, $data);
}
\end{lstlisting}

%------------------------------------------------------------------------------
\subsection{\Class{execMethod} function}
\label{app:fence:gitlab:execmethod}

\begin{lstlisting}
private function execMethod($method, $endPoint, $data = null)
{
    $this->init($endPoint);
    $this->setMethod($method);
    if ($data) {
        $this->setBodyData($data);
    }

    return $this->exec();
}
\end{lstlisting}

%------------------------------------------------------------------------------
\subsection{\Class{createProject} function}
\label{app:fence:gitlab:createproject}

\begin{lstlisting}
public function createProject($project, $parameters = [])
{
    $name = $project;
    if ($project instanceof Project) {
        $name = $project->name();
    }

    \FENCE\Logger::debug("Creating project = {project}", ["project" => $project]);
    $payload = $this->post('projects', array_merge([
        'name' => $name
    ], $parameters));

    if (! isset($payload['id'])) {
        throw new Exception\ProjectAlreadyExistsException(
            json_encode($payload)
        );
    }

    return new Project($payload['id'], $payload);

}
\end{lstlisting}
