# Supplementary material for: A continuous integration and web framework in support of the ATLAS Publication Process
Source: arXiv:2005.06989 source file (2021-01-28)
Supplement: Supplementary file 3 [file Appendix_authorlist.tex]

%------------------------------------------------------------------------------
\section{Author list files}%
\label{app:authorlist}
%------------------------------------------------------------------------------
