# Supplementary material for: A continuous integration and web framework in support of the ATLAS Publication Process
Source: arXiv:2005.06989 source file (2021-01-28)
Supplement: Supplementary file 4 [file Appendix_proofs.tex]

%------------------------------------------------------------------------------
\section{Proofs checks}%
\label{app:proofs}
%------------------------------------------------------------------------------
